# Supplementary material for: Direct Consistency Optimization for Robust Customization of Text-to-Image Diffusion Models
Source: arXiv:2402.12004 source file (2024-12-12)
Supplement: Supplementary file 1 [file appendix_user_evaluation.tex]

\begin{figure}[t]
    \centering
    \begin{subfigure}{0.99\textwidth}
    \includegraphics[width=\linewidth]{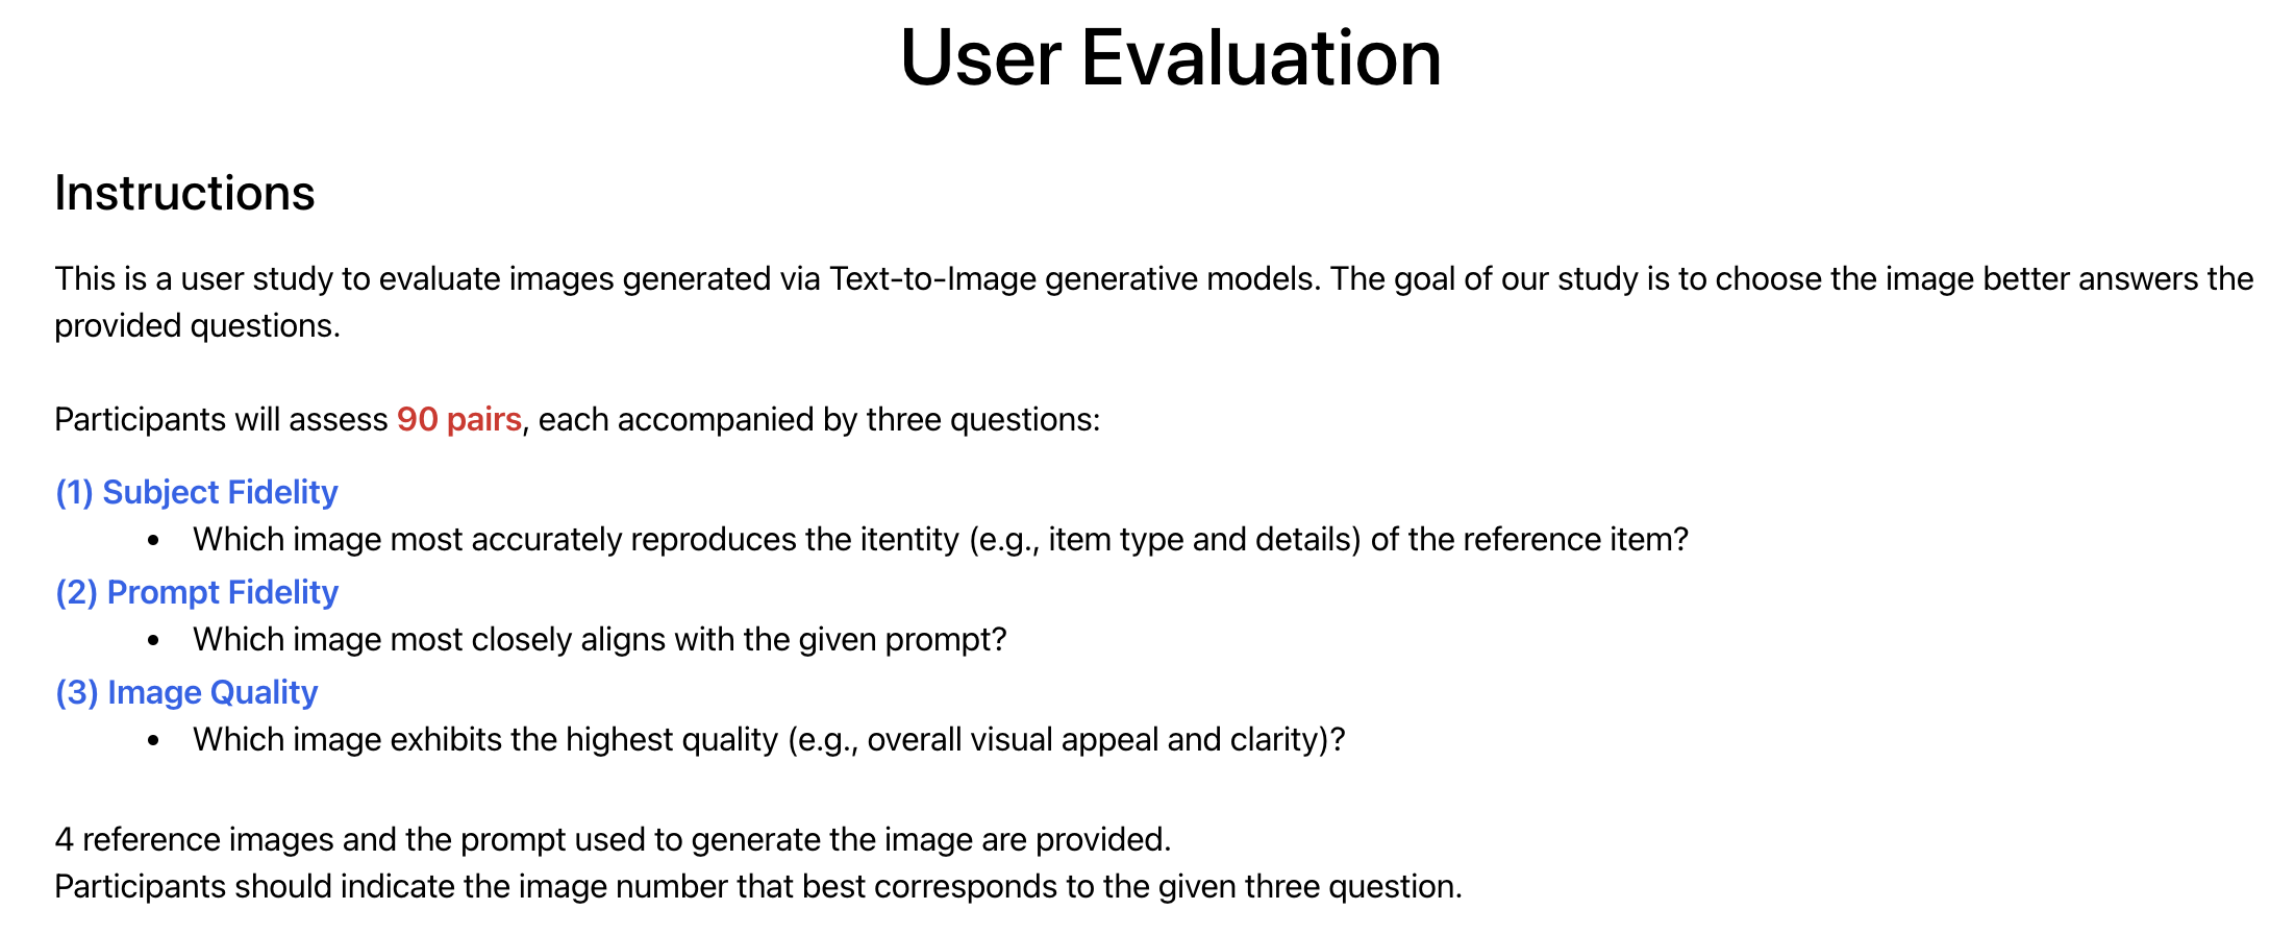}
    \vspace{-0.2in}
    % \caption{User instructions}
    \label{fig:user_instruction}
    \end{subfigure}
    \hfill
    \begin{subfigure}{0.99\textwidth}
    \includegraphics[width=\linewidth]{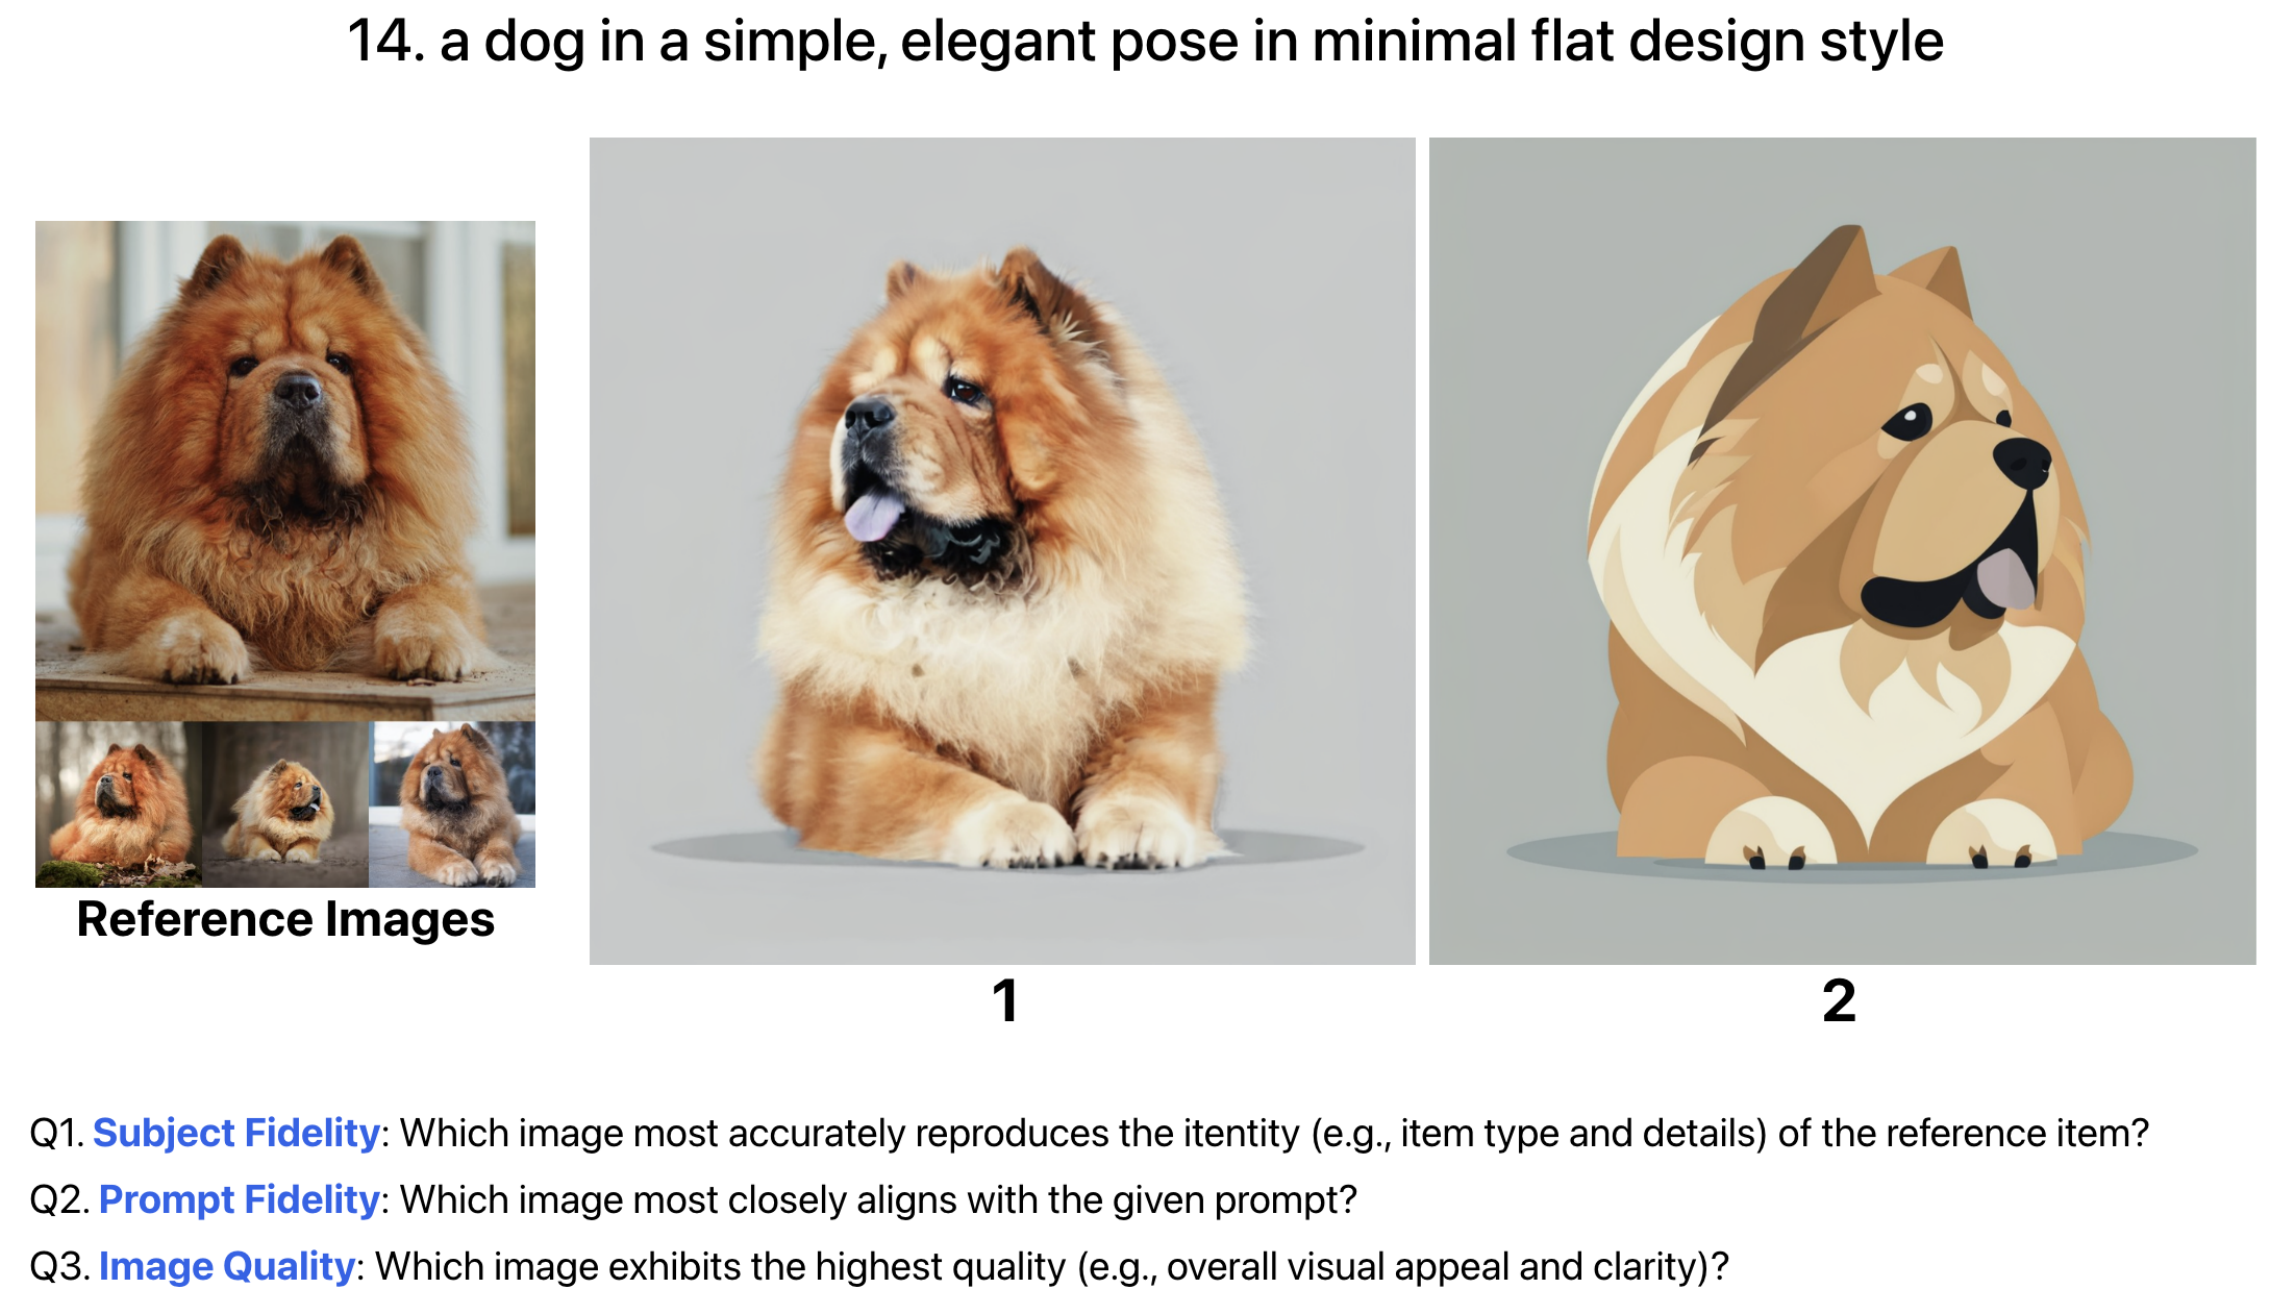}
    \vspace{-0.2in}
    % \caption{Example of user study interface}
    \label{fig:user_interface}
    \end{subfigure}
    \caption{User preference study interface. We ask users to choose one from two images that is better aligned with the subject reference image or the text prompt or demonstrates better image quality.}
    \label{fig:user_study}
    \vspace{-5pt}
\end{figure}

% \begin{figure*}[ht]
%     \small\centering
%     \includegraphics[width=\textwidth]{resources/appendix/user_study_2.pdf}
%     \vspace{-5pt}
%     % \caption{}
%     \label{fig:user_study_1}
% \end{figure*}

% % \begin{figure*}[ht]
% %     \small\centering
% %     \includegraphics[width=\textwidth]{resources/appendix/user_study_2.pdf}
% %     \vspace{-5pt}
% %     \caption{
% %     User preference study interface. We ask users to choose one from two images that is better aligned with the subject reference image or the text prompt or demonstrates better image quality. }
% %     \label{fig:user_study_2}
% % \end{figure*}
